# Supplementary material for: Robust Parahydrogen-Induced Polarization at High Concentrations
Source: arXiv:2401.07243 source file (2024-01-14)
Supplement: Supplementary file 1 [file SI_appendix.tex]

\subsection*{Details regarding the effective Hamiltonian reached via Average Hamiltonian Theory} \label{seq:SI-AHT}
In \ref{sec:theoryDNP}, we referred to a "suitable choice" for $B_1(t)$ to reach \eqref{eq:pol-transfer-H-eff} from \eqref{eq:pol-transfer-H} by applying Average Hamiltonian Theory.
Here, we provide a complete calculation using the SLIC sequence as an example.

In the lab frame, the system is described by the Hamiltonian from \eqref{eq:pol-transfer-H}:
\begin{align}
    H(t) = \omega_I \hat{I}_z + \omega_S \hat{S}_z + A_\perp \hat{I}_x  \hat{S}_z + \gamma_S B_1(t)\hat{S}_x. 
\end{align}
Here, $B_1(t) = 2\Omega(t)/\gamma\ \cos(\omega_{B1} t + \varphi(t))$ describes our linearly polarized driving field which oscillates with angular frequency $\omega_{B1}=\omega_S-\Delta$ where the resonance offset $\Delta$ is usually unintended.

We can now enter the frame corotating with the Larmor precessions (except for $\Delta$) using $H^{\text{L}}=\omega_{B1} \hat{S}_z + \omega_I \hat{I}_z$ and the corresponding unitary $U^{\text{L}} = e^{-i \omega_{B1} t \hat{S}_z} e^{-i \omega_{I} t \hat{I}_z} $ and reach
\begin{align}
    H^L(t) &\approx  \Delta \hat{S}_z + A_\perp (\hat{I}_x \cos(\omega_I t) - \hat{I}_y \sin(\omega_I t))  \hat{S}_z \nonumber \\ 
    &+ \Omega(t) (\cos\varphi(t)\hat{S}_x+ \sin\varphi(t)\hat{S}_y),
\end{align}
where we discarded terms oscillating with $2\omega_{S}$ using the scale hierarchy \eqref{eq:scale_hierarchy}. In regimes where $B_0$ is weaker, the use of rotating waves for $B_1$ avoids the need for this approximation.
Finally we can enter the frame corotating with the influence of our drive, also called the toggling frame, as defined by 
\begin{equation}
    U(0)=\mathbb{1}, \ i\partial_t U(t) =  \Omega(t) (\cos\varphi(t)\hat{S}_x+ \sin\varphi(t)\hat{S}_y) + \Delta \hat{S}_z.
\end{equation}
In this frame, only the interaction between the spins remains part of the Hamiltonian
\begin{align}
    H^{\text{tog}}(t) &= A_\perp (\hat{I}_x \cos(\omega_I t) - \hat{I}_y \sin(\omega_I t)) U^\dagger(t) \hat{S}_z U(t) \nonumber \\
    &=:A_\perp (\hat{I}_x \cos(\omega_I t) - \hat{I}_y \sin(\omega_I t)) \hat{S}^{\text{tog}}_z(t).
\end{align}
Here, we used that $U(t)$ commutes with the spin $I$ operators and defined the toggling-frame $\hat{S}_z$ operator $\hat{S}^{\text{tog}}_z(t)$. Thanks to $A_\perp \ll \omega_I$ we can now approximate the Hamiltonian $H^{\text{tog}}(t)$ with its time average over a duration $T\sim 2\pi/\omega_I$ and reach a constant effective Hamiltonian. For this we assume that the chosen drive returns the state of $S$ to its original state at time $T$, i.e. $U(T)=U(0)$, and the same for the Larmor precession on spin $I$, that is $\exp{i\omega_I T} = 1$. This ensures that the same effective Hamiltonian describes the time spans $[0,T]$, $[T,2T]$ et cetera for as long as the same driving sequence is applied. The effective Hamiltonian becomes
\begin{align}
    H^{\text{eff}} &= \dfrac{1}{T}\int_0^T \mathrm{d} t\ H^{\text{tog}}(t) \\
        &= A_\perp\ \dfrac{1}{T}\int_0^T \mathrm{d} t\ (\hat{I}_x \cos(\omega_I t) - \hat{I}_y \sin(\omega_I t)) \hat{S}^{\text{tog}}_z(t). \nonumber
\end{align}
It becomes apparent that $H^{\text {eff}}$ contains an $\hat{I}_x$ component proportional to the frequency-$\omega_I$ cosine contribution of $\hat{S}^{\text{tog}}_z(t)$ and similarly for $\hat{I}_y$ and the $\omega_I$ sine contribution of $\hat{S}^{\text{tog}}_z(t)$.

In case of SLIC, we describe the initial and final pulses as instant at times $t=0$ and $t=NT$ respectively, such that
\begin{align}
    \hat{S}^{\text{tog}}_z(0^-) &= \hat{S}_z \nonumber \\
     \overset{\left(\pi/2\right)_{Y}}{\rightarrow} & \hat{S}^{\text{tog}}_z(0^+) = U^{\text{ini}\dagger}(0^+) \hat{S}_z U^{\text{ini}}(0^+) = - \hat{S}_x \\
   & U^{\text{ini}}(0^+) = \cos(\pi/4)\mathbb{1}+i\sin(\pi/4) 2 \hat{S}_y.
\end{align}
As the duration of this pulse is negligible, we need not regard any corresponding effective Hamiltonian here.

During the spin-locking pulse of SLIC, we have $(\Omega(t),\varphi(t)) = (\omega_I, 0)$, which leads to $U(t)=\exp{(-i\omega_I t \hat{S}_x)} = \cos(\omega_I t/2) \mathbb{1}+ i\sin(\omega_I t/2) 2\hat{S}_x$.
This gives us 
\begin{align}
\hat{S}^{\text{tog}}_z(t) &= U^{\text{ini}\dagger}(0^+) U^\dagger(t) \hat{S}_z U(t) U^{\text{ini}}(0^+) \\
&= U^{\text{ini}\dagger}(0^+) ( \cos(\omega_I t) \hat{S}_z + \sin(\omega_I t) \hat{S}_y ) U^{\text{ini}}(0^+) \nonumber \\
&= -\cos(\omega_I t) \hat{S}_x + \sin(\omega_I t) \hat{S}_y, \nonumber
\end{align}
which together with $T=2\pi/\omega_I$ leads to the effective Hamiltonian
\begin{align}
    H^{\text{eff}}_{SLIC} &= A_\perp\ \dfrac{1}{T}\int_0^T \mathrm{d} t\ (\hat{I}_x \cos(\omega_I t) - \hat{I}_y \sin(\omega_I t)) \hat{S}^{\text{tog}}_z(t) \nonumber \\
    &= A_\perp \left( \dfrac{ -\hat{I}_x \hat{S}_x - \hat{I}_y \hat{S}_y}{2} \right),
\end{align}
which now corresponds to a flip-flop interaction. The opposite sign compared to \eqref{eq:pol-transfer-H-eff} does not change its properties with regards to our purposes.
The final $\pi/2$ pulse is now needed to let the toggling frame coincide with the frame $L$ if the final state of $S$ is of importance.

\subsection*{Details of the Hamiltonian equivalence}
In \cref{seq:th_pol_transfer_PHIP}, we introduce the pseudo-spin basis $(I\oplus \tilde{I})\otimes S$ to arrive at the 
Hamiltonian given in \cref{eq:phip_new_full} which, in turn, is equivalent to the Hamiltonian in the DNP setting if 
restricted to the $I\otimes S$ subspace. Here, we provide the intermediate steps of the required calculations. 

We define the pseudo-spin operators $I_z = (\ket{T_0}\bra{T_0}-\ket{S_0}\bra{S_0})/2$, 
$I_x = (\ket{T_0}\bra{S_0}+\ket{S_0}\bra{T_0})/2$ and $\tilde{I}_z= (\ket{T_{+1}}\bra{T_{+1}}-\ket{T_{-1}}\bra{T_{-1}})/2$. 
For their squares we find

\begin{align}  
	I_z^2 = \dfrac{1}{4}(\ket{T_0}\bra{T_0}+\ket{S_0}\bra{S_0}) =: \frac{1}{4}\hat{P}_{\tilde{I}}
\end{align} 
and
\begin{align} 
	\tilde{I}_z^2 = \dfrac{1}{4}(\ket{T_{+1}}\bra{T_{+1}}+\ket{T_{-1}}\bra{T_{-1}}) =: \frac{1}{4}\hat{P}_I
\end{align}
with the respective projectors $\hat{P}_I$ and $\hat{P}_{\tilde{I}}$ onto subsystems $I$ and $\tilde{I}$ in the 
Hydrogen-manifold. Note that in this pseudo-spin basis, all operators in $I\oplus \tilde{I}$ need to be considered 
as acting on the full 4-level Hydrogen-manifold. In contrast, the original basis $I^{(1)}\otimes I^{(2)}$ allows 
the corresponding operators to be considered as true single-spin operators due to the tensor-product structure.

The $J$-coupling contribution can now be expressed in the new basis, resulting in
\begin{align} 
	\hat{\vec{I}}^{(1)}\cdot\hat{\vec{I}}^{(2)} &= \dfrac{1}{4}(\ket{T_{+1}}\bra{T_{+1}}+\ket{T_{0}}\bra{T_{0}}+\ket{T_{-1}}\bra{T_{-1}}) \nonumber\\
	& \quad - \dfrac{3}{4} \ket{S_{0}}\bra{S_{0}} \nonumber\\
	&= \dfrac{1}{4}(\ket{T_{+1}}\bra{T_{+1}}+\ket{T_{-1}}\bra{T_{-1}}) \nonumber \\
	& \quad -\dfrac{1}{4}(\ket{T_{0}}\bra{T_{0}}+\ket{S_{0}}\bra{S_{0}}) \nonumber\\
	&\quad +\dfrac{1}{2} (\ket{T_{0}}\bra{T_{0}}-\ket{S_{0}}\bra{S_{0}}) \nonumber\\
	&= \frac{1}{4}\hat{P}_{\tilde{I}} - \frac{1}{4}\hat{P}_I + \hat{I}_z.
\end{align}
Finally the $\hat{I}^{(i)}_z$ operators become
\begin{align}
	\hat{I}^{(1)}_z \otimes \hat{\mathbb{1}}^{(2)} &= \dfrac{1}{2} ( \ket{S_{0}}\bra{T_{0}}+\ket{T_{0}}\bra{S_{0}} \nonumber \\
 &\qquad +\ket{T_{+1}}\bra{T_{+1}}-\ket{T_{-1}}\bra{T_{-1}} ) \nonumber \\ 
	&=\hat{I}_x+\hat{\tilde{I}}_z, \\ 
	\hat{\mathbb{1}}^{(1)} \otimes \hat{I}^{(2)}_z &= \dfrac{1}{2} ( -\ket{S_{0}}\bra{T_{0}}-\ket{T_{0}}\bra{S_{0}}  \nonumber \\
 &\qquad +\ket{T_{+1}}\bra{T_{+1}}-\ket{T_{-1}}\bra{T_{-1}} ) \nonumber \\
	&=-\hat{I}_x+\hat{\tilde{I}}_z. 
\end{align}

With these results, we can directly replace all contributions to the Hamiltonian from \cref{eq:PHIP_bare} to reach
\begin{align}
	H &= \omega^0_I \hat{I}^{(1)}_z +\omega^0_I \hat{I}^{(2)}_z +\omega_S \hat{S}_z + J\,\hat{\vec{I}}^{(1)}\cdot\hat{\vec{I}}^{(2)} \nonumber \\ 
	&\quad + J^{(1)} \hat{S}_z \hat{I}^{(1)}_z+J^{(2)} \hat{S}_z \hat{I}^{(2)}_z \nonumber \\
	&= 2\omega^0_I\hat{\tilde{I}}_z + \omega_S \hat{S}_z  + \frac{J}{4}\,(\hat{P}_{\tilde{I}} - \hat{P}_I + 4\hat{I}_z) \nonumber \\
	&\quad + \frac{1}{2}(J^{(1)}+J^{(2)}) S_z \hat{P}_{\tilde{I}} + (J^{(1)}-J^{(2)}) S_z I_x \nonumber \\
	&=  J  \hat{I}_z + \omega_S \hat{S}_z +  (J^{(1)}-J^{(2)}) \hat{S}_z \hat{I}_x  \nonumber \\
	&\quad + 2\omega^0_I\hat{\tilde{I}}_z + \frac{J}{4}\hat{P}_{\tilde{I}} - \frac{J}{4}\hat{P}_I + (\dfrac{J^{(1)}+J^{(2)}}{2}) \hat{P}_{\tilde{I}} \hat{S}_z,
\end{align}
where all terms in the second line commute with all terms in the first line and the former becomes equivalent to \cref{eq:pol-transfer-H} if restricted to the $I\otimes S$ subspace.

\subsection*{Details of the numerical simulation}

The numerical simulations in this work use the pseudo-spin basis $I \otimes S$ for the Hamiltonian. The drive is 
parametrized via a time-dependent amplitude $\Omega(t)$ and phase $\varphi(t)$:
\begin{align*}
	H(t)&= \omega_I \hat{I}_z +A_\perp\hat{S}_z\hat{I}_x \\ 
	&\quad + (1+\dfrac{\Omega_{error}}{\Omega})\cdot \Omega(t)\left( \cos(\varphi(t)) \hat{S}_x + \sin(\varphi(t))\hat{S}_y \right) \\ &\quad + \Delta\hat{S}_z.
\end{align*}
Here, $\Omega_{error}/\Omega$ is the relative error in the Rabi frequency created by the drive on spin $S$, 
and $\Delta$ parametrizes resonance-offset errors of the drive. The system state starts in the state
$$\rho = |+\frac{1}{2}\rangle\langle +\frac{1}{2}|\otimes \frac{1}{2}\hat{\mathbb{1}}$$ where $\hat{I}_z|+\frac{1}{2}\rangle=\frac{1}{2}|+\frac{1}{2}\rangle$. 

The integration in time of the dynamics is governed by the piece-wise constant Hamiltonian $H(t)$. It proceeds by direct exponentiation of the Hamiltonian in each interval where it is constant and chooses, where 
applicable, the number of sequence repetitions $N$ such that the first maximum of the $S$-magnetization is 
reached for the error-free case of $\Omega_{error}=\Delta=0$. For schemes which do not rely on sequence
repetition such as amplitude sweeps and the non-repeating variant of S2hM, $N=1$ is chosen whereas the
duration of the sequence, i.e. the sweep duration or the lengths of the pulse trains, is given by the theoretically optimal values. For the robustness-plots, this value of $N$ is used for calculating the polarization 
reached for a variety of errors in $\Omega_{error}/\Omega$ and $\Delta/\Omega$ and the final polarization is
calculated via the expectation value $\langle S_z\rangle$.

The timing of pulses is calculated in two steps: First, the total duration of a sequence iteration is calculated 
as a sequence-dependent multiple of the Larmor period $\tau$. Secondly, the individual pulses of rotation angle 
$\alpha_i$ and durations $T_i = \alpha_i/\Omega_i$ are distributed in the time interval such that pulses begin 
and end together with their corresponding section defined by $\tau$. Unless specified differently by the sequence, 
the pulses have equal interpulse waiting times to optimize refocusing of rotations induced by $\Delta$. Unless specified otherwise by the polarization
scheme, the maximum Rabi frequency $\Omega(t)=\Omega_i =\Omega$ is assumed to be used for the duration of each 
pulse $i$.

\subsection*{Description of robustness properties}
The intended effective Hamiltonian for polarization transfer between the spins $S$ and $I$ is given by 
\cref{eq:pol-transfer-H-eff} and contains only the Larmor precession of the two spins together with a 
flip-flop contribution of strength $A_\ast \le A_\perp$.

For a full polarization transfer, it is necessary that any accumulating errors which alter the spin state 
remain small over the whole duration $T=2\pi/A_\ast$. For non-error-correcting sequences, unwanted 
Hamiltonian contributions such as a resonance offset $\Delta\hat{S}_z$ will accumulate at an error rate 
$\alpha=\Delta$, whereas first order error-correction due to a drive of Rabi frequency $\Omega$ can suppress 
this to $\alpha \propto (\Delta/\Omega)^2\cdot \omega_I$ where $(\Delta/\Omega)^2$ estimates the scaling 
behavior of the error accumulated during a single repetition of the error-correcting part of the sequence 
and $\omega_I\propto 1/\tau$ estimates the duration of that sequence part.

Thus, for an error of strength $\beta$ and a non-correcting sequence, successful polarization transfer is assured for 
\begin{align}
	\beta = \alpha \ll A_\ast,
\end{align}

and in the case of a (first-order) robust sequence for
\begin{align}
	  c\,(\beta/\Omega)^2\cdot \omega_I = \alpha \ll A_\ast \Leftrightarrow \beta \ll c\, \Omega \sqrt{\dfrac{A_\ast}{\omega_I}},
\end{align}
where $c$ is a proportionality constant depending on the sequence and the details of the type of the error. 
In the main text, we refer to the former as "maximum acceptable error scaling with $A_\perp$" and to the 
latter as "maximum acceptable error scaling with $\Omega$". Note that the latter case still includes an 
additional square root scaling with $A_\perp$.

The errors we regard in this work are detuning errors $H_{err}=\Delta\hat{S}_z$ of the driving field with 
$\beta=\Delta$, and Rabi errors 
\begin{align}
    H_{err}(t)&=\dfrac{\Omega_{error}}{\Omega}\cdot \Omega(t)\left( \cos\varphi(t) \hat{S}_x + \sin\varphi(t)\hat{S}_y \right) 
\end{align}
with $\beta = \Omega_{error}$.

\subsection*{Details of the regarded polarization schemes}

Here, we provide further details about the sequences and robustness properties of the schemes under consideration 
in their respective parameter regimes.

The more general robustness plots in Fig.~\ref{fig:SI_app_1} show the robustness properties of the sequences for 
different regimes of the scale hierarchy $\Omega,\omega_I\gg A_\perp$. From left to right, the coupling between 
the spins $A_\perp$ decreases; from top to bottom $\omega_I$ decreases. 
All results shown remain in the regime $\Omega>\omega_I$. Still, one observes that different sequences display comparative 
advantages in different parameter regimes. All of the robustness plots show the duration $t_{fin}$ of the sequence
compared to a reference given by the ideal application of SLIC $t_{fin}^{SLIC}=2\pi/A_\perp$. Note that these times 
are not necessarily the optimal choices as the algorithm for choosing $N$ is quite simple, and additionally for 
SLIC/NOVEL and ADAPT/TOP-DNP the duration for a single repetition was chosen to correspond to a total rotation angle 
of $2\pi$ although the sequences allow for a finer decomposition. Due to this, the resulting values for $t_{fin}$ as 
well as the calculated robustness properties are less representative of the corresponding sequences in the regime 
$A_\perp \approx \omega_I$, i.e. the lower-left corner of Fig.~\ref{fig:SI_app_1}b,d,f,h,j and m.

\paragraph{SLIC and NOVEL.} This scheme (cf. \cref{fig:SI_app_1} a,b) consists of initial and final $\pi/2$ pulses to 
switch from the $+z$-orientation to the $+x$-orientation (and back) and an intermediate spin-locking pulse with 
amplitude $\Omega = \omega_I$ and phase $X$. In order to treat this scheme as a pulsed scheme, we restricted the 
spin-locking pulse to $N$ repetitions of a pulse of rotation angle $2\pi$ (Fig.~\ref{fig:SI_app_1}a). In Fig.~\ref{fig:SI_app_1}b, 
one can clearly see that close to the error-free point of $\Delta=0=\Omega_{error}$, acceptable amplitude errors 
$\Omega_{error}$ are limited by $A_\perp$ , whereas detuning errors $\Delta$ may reach larger values proportional 
to the amplitude of the spin-locking pulse $\omega_I$. As the amplitude of this pulse is fixed by the spin system, 
it is not possible to take advantage of larger possible values for $\Omega$.

\paragraph{ADAPT and TOP-DNP.} For simplicity and comparability, we only consider the versions with $\pi/2$ pulses and 
stay in the regime of $\Omega>\omega_I\gg A_\perp$. For the regime of $\Omega<\omega_I$ or $\omega_I \sim A_\perp$ 
we refer to the original works \cite{Stevanato2017b,Tan2019}. Choosing $\tau= \pi/(2\omega_I)$, each repetition 
of the sequence consists of four $\pi/2$ pulses of phase $X$ with pulse-to-pulse delay $\tau$. Again, initial and final 
pulses are $\pi/2$ pulses with phases $Y$ and $-Y$ and suitable waiting times such that any two subsequent pulses have 
equal waiting times (cf. Fig.~\ref{fig:SI_app_1}c). The robustness properties of this sequence are shown in Fig.~\ref{fig:SI_app_1}d 
and show a central robust region very similar to that of SLIC/NOVEL, however with additional sidebands in $\Delta$ 
repeating over a region proportional to the Rabi amplitude $\Omega$.

\paragraph{S2hM and NV nuclear initialization} In the main text, we presented the properties of an S2hM variant with 
a fixed pulse train length of $n=8$ $\pi$-pulses
and adjusted waiting times in order to enable phase cycling and full rephasing without 
adjustments to the specific values of $\omega_I$ and $A_\perp$. Comparable robustness properties are still achievable with 
a repetition-free version of S2hM (i.e. $N=1$) as long as phase cycling is used and additionally all waiting times are refocussed 
by $\pi$-pulses. S2hM uses the same initial and final $\pi/2$ pulses of phases $Y$ and $-Y$ as SLIC/NOVEL, and the main 
part of the sequence consists of two pulse trains of $n$ $\pi$-pulses, each surrounded by symmetric waiting times of length 
$\tau/2$ (which together include the pulse-duration) and a transitory $\pi/2$ pulse of phase $X$ together with an extra 
waiting time of $\tau/2$. The time scale of $\tau$ is given by $\tau = \pi/\omega_I$. 
In the robust repeating version of S2hM used in the main text, the $\pi$-pulse trains each consist of four pulses, the 
first with phases $X,Y,X,Y$ and the second with phases $Y,X,Y,X$. To achieve refocusing of all waiting times for any 
number of repetitions $N$, the extra waiting time of $\tau/2-\pi/(2\Omega)$ after the transitory $\pi/2$ pulse 
is separated into two equal parts with the second part being added to the waiting time between the third and fourth 
pulse of the second pi train (cf. Fig.~\ref{fig:SI_app_1}c). Note that for a single repetition $N=1$, this sequence is 
fully equivalent to a usual S2hM sequence with $n=4$ $\pi$-pulses per train and slightly unusual waiting times. For more repetitions ($N>1$), the additional pulse trains per repetition each correspond to a single longer pulse train of $n=8$ $\pi$-pulses with $XY8$ phases. As can be seen in 
Fig.~\ref{fig:SI_app_1}f, this choice allows for $\Omega$-scaling of acceptable errors in both $\Omega_{error}$ and $\Delta$.

As an example for the robustness properties of S2hM without phase cycling, we regard a simpler sequence of equal pulse trains which each consist of $n= \lfloor\dfrac{\pi \omega_I}{2 A}_\ast\rceil$ pulses of equal phase $X$, where $\lfloor \cdot \rceil$ rounds to the closest integer. The waiting time after the transitory $\pi/2$ pulse of phase $X$ is chosen such that the delay between the two pulse trains is $\tau/2$. Finally, an equal waiting time is added before the final $\pi/2$ pulse in order to refocus rotations induced by $\Delta$ during the intermediary waiting times at least in the cases where $N$ is an odd integer (cf. Fig.~\ref{fig:SI_app_1}k). As can be seen in Fig.~\ref{fig:SI_app_1}l, this version of S2hM is susceptible to Rabi errors $\Omega_{error}$, and while the robustness to detuning errors $\Delta$ does scale with $\Omega$, it is still significantly weaker than that of the phase cycled version or that of PulsePol.

\paragraph{PulsePol} In PulsePol, the initial and final pulses are already included in the basic blocks that are repeated 
in the sequence. This part consists of two equal blocks which only differ by a phase shift of all pulses by $\varphi=\pi/2$. 
The first block consists of a central $\pi$ pulse of phase $X$, surrounded by two equal waiting times and begins and ends 
with a $\pi/2$ pulse of phase $Y$. The total duration of a block is $\tau/2$ (cf. Fig.~\ref{fig:SI_app_1}g), while the 
optimal resonance condition is $\tau= 3\pi/\omega_I$. As can be seen in Fig.~\ref{fig:SI_app_1}h, PulsePol retains successful 
polarization transfer in a large uniform region scaling with $\Omega$ both for Rabi ($\Omega_{error}$) and detuning ($\Delta$) 
errors. At a slight cost to the speed of the sequence, it is possible to increase the robust region further by using 
$\varphi=\pi/4$ and $\tau=3.5 \pi/\omega_I$ instead \cite{Tratzmiller2021}.

\paragraph{Adiabatic $B_1$ sweeps} Similar to SLIC/NOVEL, the amplitude sweep consists of initial and final $\pi/2$ 
pulses of phases $Y$ and $-Y$. The main part consists of a continuous pulse with linearly increasing amplitude, 
here $\Omega\in [0.6\,\omega_I,\ 1.4\,\omega_I]$. In our case, this pulse is approximated by 150 pulses of constant 
amplitude each (cf. Fig.~\ref{fig:SI_app_1}i). The total duration of the swept pulse is given by 
$(1.4\,\omega_I-0.6\,\omega_I)/\dot\Omega =\frac{(2\pi)}{A_\perp^2} \cdot 0.8\, \omega_I$. The robustness properties are very 
similar to the ones of SLIC/NOVEL except for the significantly improved robustness to amplitude errors (cf. Fig.~\ref{fig:SI_app_1}j).

\begin{figure*}
   	\centering
   	\includegraphics[width=\linewidth]{figures/Fig_SI_1_grid_v4.pdf}
   	\caption{Detailed robustness plots for all sequences. The sequences are shown in (a,c,e,g,i,k) and the corresponding robustness plots in different regimes of $A_\perp, \omega_I, \Omega$ are shown in (b,d,f,h,j,l). In the robustness plots, from left to right $A_\perp$ and from top to bottom $\omega_I$ is decreased by a factor of 2 in each step and each heatmap shows the success of polarization transfer over varying detuning $\Delta$ and amplitude errors $\Omega_{error}$.
    a,b) show the SLIC sequence (NOVEL in DNP),
    c,d) show the ADAPT sequence in the case of PHIP and TOP-DNP in the case of DNP. The chosen pulse duration corresponds to a $\pi/2$ pulse and the resonance condition equivalent to SLIC/NOVEL was used.
    e,f) show the S2hM sequence with a fixed n=8 XY8 phase cycle and the waiting time distributed equally before the first and fourth $\pi$ pulse after the $\pi/2$ pulse. The corresponding results for S2hM with fixed phases are shown in k,l).
    g,h) show PulsePol,
    i,j) show a linear $B_1$ sweep with $\Omega\in[0.6\omega_I,\ 1.4\omega_I]$. The duration of the swept pulse in (i) is not to scale.
    k,l) show the S2hM sequence with without phase cycling. The corresponding results for S2hM with XY8 phases are given in the e,f).
    }
    \label{fig:SI_app_1}
\end{figure*}
